# Supplementary material for: Symmetry-Informed Governing Equation Discovery
Source: arXiv:2405.16756 source file (2024-11-04)
Supplement: Supplementary file 1 [file misc.tex]

\section{Miscellaneous}

\subsection{Derivation of Lie symmetries for L-V system}

Consider the Lotka-Volterra system governed by
\begin{equation}
    \left\{
    \begin{aligned}
    \dot{p} &= p(a-q) \\
    \dot{q} &= q(p-b)
    \end{aligned}
    \right.
\end{equation}

For simplicity, we use the above equation form with $p$ and $q$ standing for the population density rather than \eqref{eq:lv} in the main paper with logarithm densities as state variables. Also, we remove two of the free coefficients in the equations, so the $pq$ terms have fixed coefficients $1$. Equations with arbitrary coefficients for cross terms can be recovered by a rescaling on $p$ and $q$. These changes would affect the analytic expression of the symmetries but not the structure of the symmetry group (e.g. the number of infinitesimal generators).

% Assume the symmetries are time-independent, i.e. $v = \phi_p(p, q)\partial_p + \phi_q(p, q)\partial_q$. From the infinitesimal criterion (\cref{th:lps-inf}), we have the determining equations for the Lie symmetries:
% \begin{align}
%     & p(a-q) \partial_p \phi_p + q(p-b) \partial_q \phi_p - (a-q) \phi_p + p \phi_q = 0 \\
%     & p(a-q) \partial_p \phi_q + q(p-b) \partial_q \phi_q - q \phi_p - (p-b) \phi_q = 0
% \end{align}

We can convert the system of equations to a single second-order equation by eliminating $q$. From the first equation,
\begin{equation}
    q = \frac{1}{p}(ap - \frac{dp}{dt}).
\end{equation}

Substituting this expression into the first equation and simplifying it, we have
\begin{equation}
    \Delta = \ddot p + (b - p) \dot p - \dot p^2 / p - abp + ap^2 = 0.
\end{equation}

Assume the symmetries take an evolutionary form, i.e.
\begin{equation}
    \mathbf v = \phi(p, \dot p, t) \frac{\partial}{\partial p}
\end{equation}

According to the infinitesimal criterion,
\begin{equation}
    \mathrm{pr}^{(2)} \mathbf v [\Delta] \big | _ {\Delta = 0} = 0, \label{eq:lie-symm-det-eq}
\end{equation}
where the prolonged vector field can be computed from the prolongation formula (Th 2.36, \citet{olver1993applications})
\begin{equation}
    \mathrm{pr}^{(2)} \mathbf v = \phi \frac{\partial}{\partial p} + D_t \phi \frac{\partial}{\partial \dot p} + D_t^2 \phi \frac{\partial}{\partial \ddot p}. \label{eq:prolongation-formula}
\end{equation}

It is at this point that we need some additional assumptions about $\phi$. Otherwise, it would be too hard to solve the determining equation \eqref{eq:lie-symm-det-eq} for a general function $\phi$.

For example, we can assume $\phi$ is linear in $\dot p$:
\begin{align}
    \phi &= f_1(p,t) + f_2(p,t) \dot p \\
    D_t \phi &= \pd{f_1}{t} + \pd{f_1}{p}\dot p + \left(\pd{f_2}{t} + \pd{f_2}{p}\dot p\right) \dot p + \ddot p f_2\\
    D_t^2 \phi &= \pdd{f_1}{t} + 2\frac{\partial^2 f_1}{\partial p \partial t} \dot p + \pdd{f_1}{p} \dot p^2 + \pd{f_1}{p}\ddot p \cr
    &+ \left(\pdd{f_2}{t} + 2\frac{\partial^2 f_2}{\partial p \partial t} \dot p + \pdd{f_2}{p} \dot p^2 + \pd{f_2}{p}\ddot p \right) \dot p \cr
    &+ 2\left(\pd{f_2}{t} + \pd{f_2}{p}\dot p\right) \ddot p + \dddot p f_2
\end{align}

Then, substituting it into \eqref{eq:lie-symm-det-eq}:
\begin{equation}
    \phi (\dot p ^2 / p ^2 -\dot p - ab + 2ap) + D_t\phi (b-p - 2\dot p / p) + D_t^2\phi = 0
\end{equation}

We can replace all appearances of $\ddot p$ with $(p-b)\dot p + \dot p^2 / p + abp - ap^2$.

Also, $\dddot p = \dot p^2 + (p-b)\ddot p + \frac{2\dot p \ddot p}{p} - \frac{\dot p^2}{p^2} + ab\dot p - 2ap\dot p$.

Then, rearranging the above in terms of different monomials as in \cref{tab:monom-coeff}.

\begin{table}[h]
    \centering
    \begin{tabular}{cc}
    \hline
        Monomial & Coefficient \\
    \hline
        $\dot p$ & ... \\
        $\dot p ^2$ & ... \\
        $\dot p^3$ & $f_{2pp} + 3f_{2p}/p$ \\
    \hline
    \end{tabular}
    \caption{Comparing the coefficients for different monomials.}
    \label{tab:monom-coeff}
\end{table}

From $\dot p^3$, we know that $f_{2pp} + 3f_{2p}/p = 0$. Solving this equation gives us $f_2(p) = \frac{C_1}{p^2}+C_2$. As $f_2$ also depends on $t$, the general solution is
\begin{equation}
    f_2(p,t) = \frac{A(t)}{p^2} + B(t)
\end{equation}

Similarly, we can set the coefficients for $\dot p$ and $\dot p^2$ to zero and obtain other constraints. Eventually, we have the following symmetry if $a+b=0$:
\begin{equation}
    \phi = C_1 \exp (-at) (ap - \dot p) + C_2 \dot p.
\end{equation}

Then, we can recover the vector field on the original coordinate through prolongation. For instance, let $C_1=1$ and $C_2=0$:
\begin{align}
    \mathrm{pr}^{(1)}\mathbf v &= \phi\partial_p + D_t\phi \partial_{\dot p} \cr
    &= \exp(-at)pq\partial_p + (\exp(-at)pq)(-a + \dot p q + p \dot q)\partial_{\dot p}  \\
    \mathbf v |_{p,q} &= \mathrm{pr}^{(1)}\mathbf v (p) \partial_p + \mathrm{pr}^{(1)}\mathbf v (q) \partial_q \\
    &= \exp(-at) pq \partial_p - \exp(-at)pq\partial_q
\end{align}

This can be interpreted as the scaling symmetry in the phase space. I conjecture that LaLiGAN has discovered a similar symmetry as this one. However, when the phase is transformed, the time should also be rescaled. Intuitively, the trajectories with different Hamiltonians have different periods.
