# Supplementary material for: Symmetry-Informed Governing Equation Discovery
Source: arXiv:2405.16756 source file (2024-11-04)
Supplement: Supplementary file 2 [file appendix.tex]

\section{You \emph{can} have an appendix here.}

You can have as much text here as you want. The main body must be at most $8$ pages long.
For the final version, one more page can be added.
If you want, you can use an appendix like this one, even using the one-column format.

\yjk{TODO: organize the appendix.}

\section{Equation discovery with a perfect autoencoder} 
Let's assume the original space is $X\simeq \R^n$ and the latent space $Z \simeq \R^n$, having the same dimensions. 
Let the autoencoder (AE) consist of bijective encoder $\phi:X\to Z$ and decoder $\psi:Z\to X$. 
Ideally, we would have $\psi = \phi^{-1}$. 
We want to exploit the assumption of perfect AE to simplify the equation discovery process. 

Assume we have discovered a simple latent dynamics $\dot{z} = h(z)$. 
This translates to the following equation for $\dot{x}$ 
\begin{align}
    \dot{x} &= {d\over dt} \psi(z) = \grad_z \psi \dot{z} = J_\psi(z) \dot{z} \cr
    &= J_\psi(\phi(x)) \dot{z} \cr 
    &= J_\psi(\phi(x)) h(\phi(x)) 
\end{align}
When we have a perfect AE, $\psi = \phi^{-1}$, and therefore (assuming $J_\phi(x)$ is invertible)
\begin{align}
    J_\psi (z) = [J_\phi(x)]^{-1} 
\end{align}
which yields 
\begin{align}
    \dot{x} &= [J_\phi(x)]^{-1}  h(\phi(x)) 
\end{align}
This is also the equation we would have gotten if we derived $\dot{x}$ from $z = \phi(x)$, as 
\begin{align}
    \dot{z} &= J_\phi(x) \dot{x} = h(z) = h(\phi(x))\cr 
    \Rightarrow \dot{x} 
    &= [ J_\phi(x)]^{-1} h(\phi(x))
\end{align}
When the latent dynamics is linear, $h(z) = Mz = M\phi(x) $, the dynamics in the original space takes a particularly simple form 
\begin{align}
    \dot{x} = [J_\phi (x)]^{-1} M \phi(x)
\end{align}
Additionally, when $x$ and $z$ are both 2D, the form of $[J_\phi(x)]^{-1}$ is very simple and can be hand-coded.

\section{Symmetry-Based Regularization}
Applying symmetry as a hard constraint may not feasible if the action of the symmetry group is non-linear. A more general approach to utilizing the symmetry is to introduce it as a regularization. Assume the system $\dot x = f(x)$ has a symmetry group $G$, with the associated Lie algebra $\mathfrak g$. Consider any infinitesimal group action $\pi(v): \mathbb R^n \rightarrow \mathbb R^n, v \in \mathfrak g$. Slightly abusing the notation, we use $v$ to refer to both the Lie algebra element and its action $\pi(v)$ on data. We have

\begin{equation}
    \frac{\partial f(\cdot)}{\partial x}v(\cdot) - (v \circ f)(\cdot) = 0
\end{equation}

When $v$ is non-linear and cannot be represented as matrix, it is not straightforward to solve for the above constraint wrt $f$. Instead, we include it as a regularization term:

\begin{equation}
    \mathcal{L}_\text{sym} = 
    \sum_v \|\frac{\partial f(x)}{\partial x}v(x) - (v \circ f)(x)\|^2
\end{equation}

The infinitesimal action $v$ can be discovered by LaLiGAN, which decomposes the nonlinear group action as $\psi \circ \rho(v) \circ \phi$. In this formulation, we have

\begin{equation}
    v = (\frac{\partial\psi}{\partial z})^{ij}(\rho(v)z)_j\partial_i
\end{equation}

where $z = \phi(x)$.

\section{Implicit Formulation}
Assume that the governing equation is written in an implicit form \citep{sindy-pi}:
\begin{equation}
    \mathbf{ f(z,\dot z) = 0}, \mathbf z \in \mathbb R^m, \mathbf f: \mathbb R^m \rightarrow \mathbb R^m
\end{equation}

The form of the governing equation, whether explicit or implicit, does not affect our symmetry discovery algorithm. The discovered equivariance, if any, can be similarly formulated as
\begin{equation}
    \mathbf{ f(z }_t, \mathbf{ \dot z}_t) = \mathbf 0 \Rightarrow \mathbf f ( g \mathbf z_t , g \mathbf{ \dot z }_t ) = \mathbf 0
\end{equation}

We may write $g = \exp (w^iL_i)$ for a connected matrix Lie group and also $g \approx I + \epsilon^i L_i$ when $\epsilon \in \delta_0$. Then, the equivariance constraint becomes
\begin{align}
    \frac{\partial \mathbf f ( g \mathbf z , g \mathbf{ \dot z } )}{\partial \epsilon_i}
    = &
    \frac{\partial \mathbf f ( g \mathbf z , g \mathbf{ \dot z } )}{\partial (g \mathbf z)} \frac{\partial (g \mathbf z)}{\partial \epsilon_i}
    +
    \frac{\partial \mathbf f ( g \mathbf z , g \mathbf{ \dot z } )}{\partial (g \mathbf{\dot z})} \frac{\partial (g \mathbf{\dot z}))}{\partial \epsilon_i} \\
    = &
    \frac{\partial \mathbf f}{\partial \mathbf z}L_i \mathbf z + \frac{\partial \mathbf f}{\partial \mathbf{\dot z} }L_i \mathbf{ \dot z }
\end{align}

If $\mathbf f$ is expressed in terms of the function space basis as $\mathbf {f(z, \dot z)} = \mathbf \Xi \mathbf {\Theta (z, \dot z)}$, we have

\begin{equation}
    \mathbf \Xi (\mathbf{ J_\Theta (z)} L_i \mathbf z + \mathbf{ J_\Theta (\dot z)} L_i \mathbf { \dot z } ) = \mathbf 0
\end{equation}

Or, in practice, SINDy-PI seeks to minimize $\mathbf {f(z, \dot z)} = \mathbf {(I-\Xi)\Theta(z,\dot z)}$ under the constraint $\mathrm{diag}(\mathbf{\Xi}) = 0$. Thus we have

\begin{equation}
    \mathbf {(I-\Xi)} (\mathbf{ J_\Theta (z)} L_i \mathbf z + \mathbf{ J_\Theta (\dot z)} L_i \mathbf { \dot z } ) = \mathbf 0
\end{equation}

Is there a proper function space that is closed under the symmetry operator (similar to the polynomial space in the explicit formulation)? Are there any interesting examples with nontrivial symmetries?

\section{PDE Symmetries}
\subsection{Discovering Lie point symmetries}
Consider the solution of a PDE $u=f(t,x)$ where $x\in\mathbb R$. This can also be easily generalized to $\mathbf x\in\mathbb R^n$. Lie point symmetry transforms the solution to another. For instance, the spatial translation symmetry $(x,t,u)\rightarrow(x+\epsilon,t,u)$ transforms $f(t,x)$ to $f(t-\epsilon,x)$.

Infinitesimal Lie point symmetries can be represented by vector fields.
\begin{equation}
    \mathbf v = \sum_{i}\xi^i(y)\frac{\partial}{\partial y^i}
\end{equation}
where $y=(x,t,u)$ and $\xi^i$ some functions of $y$. When $\xi$ is linear, this can be represented by matrices as we did in LieGAN.

When $\xi$ is nonlinear, one possible approach may be representing $\xi$ in a function basis, as SINDy did for equation discovery. Let $W\in\mathbb R^{3\times d}$ be the weight matrix and $\mathcal D(y) \in \mathbb R^d$ be the function basis. Let $\xi = W\mathcal D(y)$.

The exponential map of $\mathbf v$ defined this way cannot be readily computed with standard matrix exponential. Two possible ways:
\begin{itemize}
    \item Use only the small transformations by first-order approximation: $e^{\epsilon\mathbf v}(y)=y+\epsilon\xi(y)$
    \item Calculate truncated Lie series expansion for larger transformations.
    \item Use ODE solver. $y'=\mathbf v(y)$
\end{itemize}

We transform all $(x,t,u)$ in one solution to another solution of the system. Then we use interpolation to get the $u$ values on the original $(x,t)$ grid.

\subsection{Deriving equation constraints from Lie point symmetries}
todo

\subsection{Or use the symmetry loss as part of the training objective}

\section{Equivariant equations}

Let $z\in \mathcal{Z}\sim \R^k$ be the latent space.
Let $\pi: G\to \GL(\mathcal{Z})$ be a representation of $G$ defining a linear action on $\mathcal{Z}$ as 
\begin{align}
    g\cdot z = \pi(g) z.
\end{align}
$\dot z\in \mathcal{Z}'$ and $\mathcal{Z}'$ is not necessarily the same as $\mathcal{Z}$.
Thus, $\dot z$ and $z$ do not necessarily transform with the same group representation. 
For instance, for a pendulum, $z$ can be the angle, meaning $z\in [0,2\pi)$, while $\dot{z}\in \R$.  
Let $\dot z$ transform with representation $\pi':G \to \GL(\mathcal{Z}')$, meaning $g\cdot \dot z = \pi'(g)z$. 

\paragraph{Symmetry condition.}
When $G $ is a symmetry of the dynamics, it must commute with $d/dt$, meaning 
\begin{align}
    \mbox{Symmetry of dynamics: }
    g\cdot {d z\over dt }= {d(g\cdot z)\over dt}.
    \label{eq:sym-cond}
\end{align}
Pick a group element $g \in G$ close to identity such that ($\eps \ll 1$)
\begin{align}
    g &= \mathrm{id} + \eps T = \mathrm{id} + \eps^a T_a \cr 
    \pi(g) &= I+\eps d\pi(T)= I+\eps L 
\end{align}
and, similarly, $\pi'(g) = I+\eps L'$. 
Here $T_a \in \mathfrak{g}= T_IG$ form an orthonormal (using the Killing form) basis for Lie algebra basis. 
$d\pi$ and $d\pi'$ are the representations of the Lie algebra induced by the group representations $\pi$ and $\pi'$, respectively. 
For brevity, we have denoted $L_a = d\pi(T_a)$ and $L_a' = d\pi'(T_a)$. 
% Denote the representations of a small element by $\pi(g) = I+\eps L$ and $\pi'(g) = I+\eps L'$.

\paragraph{Infinitesimal symmetry condition.}
Let the dynamics be 
\begin{align}
    \dot{z}= dz/dt=h(z).
\end{align}
Using first order Taylor expansion, the symmetry condition \eqref{eq:sym-cond} becomes (see app. \ref{ap:derivations-equiv-eq})
\begin{align}
    \pi'(g) \dot{z} &= h(\pi(g) z) \cr
    % (I+\eps \cdot L') \dot z &= h((I+\eps\cdot L)z) \cr 
    % &= h(z) + [\eps\cdot Lz]^i \ro_i h(z) + O(\eps^2)\cr 
    \Rightarrow L_a'\dot z&=[L_az]^T \grad h(z) 
    \label{eq:Lz-dyn-sym}
\end{align}
Defining the linear operator (vector field in $T\mathcal{Z}$). 
\begin{align}
    \hat{L}_a(z) \equiv [L_az]^i \ro_i  
\end{align}
the dynamics symmetry condition \eqref{eq:Lz-dyn-sym} becomes 
\begin{align}
    L_a' h(z) &= \hat{L}_a h(z). 
    \label{eq:inf-sym-cond}
\end{align}
% \begin{remark}
% \nd{
    % Eq. \eqref{eq:inf-sym-cond} may be a generalization of the ``continuity equations'' $d\rho + \grad \cdot J = 0 $ in physics, but it doesn't have a sum over $a$...
    % When we have an invariant dynamics, meaning $L_a h(z)=0$, we get $\hat{L}_a h(z) = 0$. 
    % When the symmetry is translation, we have $\hat{L}_a = \ro_a$ (adding a dummy dimension $z^d = 1$). 
    % }
    % Then, $\hat{L}$ 
% \end{remark}

\paragraph{Lie algebra of the vector field $\hat{L}_a$.}
Note that $\hat{L}_a$ satisfy a Lie algebra similar to that of $T_a$ (and $L_a$). 
Denote the Lie bracket relations by 
\begin{align}
    [T_a,T_b] = {f_{ab}}^c T_c
\end{align}
where ${f_{ab}}^c$ are the structure constants. 
% We have 
% \begin{align}
%     \hat{L}_a \hat{L}_b h(z)&= [L_az]^T\grad \pa{[L_bz]^T \grad h} \cr 
%     &=[L_az]^i\ro_i[L_bz]^j \ro_j h + [L_az]^i[L_bz]^j \ro_i\ro_j h \cr 
%     [L_az]^i\ro_i[L_bz]^j \ro_j h &= [L_a]^i_kz^k [L_b]^j_l \ro_iz^l \ro_j h \cr 
%     &=[L_a]^i_kz^k [L_b]^j_l \delta_i^l \ro_j h \cr 
%     &=[L_a]^i_kz^k [L_b]^j_i  \ro_j h \cr 
%     &=[L_bL_az]^T \grad h. 
% \end{align}
% The $[L_a]^i_kz^k [L_b]^j_l \ro_iz^l \ro_j f$ term is symmetric under $a\leftrightarrow b$ and cancels in the two terms from the commutator. 
Computing the action $\hat{L}_a \hat{L}_b h(z)$ of two vector fields on a scalar function $h(z)$ we arrive at the Lie algebra (see \eqref{eq:LaLb-Lie-alg})
\begin{align}
    [\hat{L}_a, \hat{L}_b]h &= \br{[L_b,L_a]z}^T \grad h %\cr 
    % & = {f_{ba}}^c\br{L_cz}^T \grad h \cr &
    = -{f_{ab}}^c \hat{L}_c h
    \label{eq:hatL-Lie-alg}
\end{align}
which is the same as the algebra satisfied by $L_a^T$. 

\nd{Because of the similar Lie algebra, maybe we can express some conditions on the dynamics $h(z)$ in terms of Linear differential operators. 
For example, instead of the simple linear dynamics $h=Kz$ where $K\in \R^{n\times n}$, we could have $h=\hat{K}z$ where $K \in T\mathcal{Z}$ is a differential operator. 
Then, maybe symmetry condition with $L=L'$ dictates that $\hat{K}$ must commute with $\hat{L}_a$, which makes it a Casimir operator? 
}

\paragraph{Example: Linear.}
In the linear case $h(z) =Kz$ we have 
\begin{align}
     [L_a' K z]_j&=
     [L_a z]^i  K_{jl} \ro_i z^l %\cr &= [L_a z]^i K_{jl} \delta_i^l = [L_a z]^i K_{ji} 
     = [KL_a z]_j\cr 
     \Rightarrow L_a' K &= KL_a
     \label{eq:KL-linear}
\end{align}
which means that $K$ has to be an intertwiner between $\pi$ and $\pi'$.  
Assuming $z$ and $\dot{z}$ transform the same way ($\pi=\pi'$), \eqref{eq:KL-linear} becomes $L_a K= KL_a$, or $[K,L_a]=0$.

\paragraph{General dynamics.}
Define the linear operator 
\begin{align}
    \hat{L}_a(z) \equiv [Lz]^i \ro_i  
\end{align}
The dynamics symmetry condition  
which defines a vector field (or flow) on $\mathcal{Z}$.  
Express $h(z) = \S \Theta(z)$ in terms of some function basis $\Theta(z)$. 
We get
\begin{align}
    L_a' h(z) &= \hat{L}_a h(z) \cr 
    [L_a' \S \Theta]_i 
    %&=[L_a']_i^j\S_j^\mu \Theta_\mu  \cr 
    % & = [L_a z]^k \ro_k \S_i^\mu \Theta_\mu(z) \cr 
    % & = \S_i^\mu [L_a z]^k \ro_k \Theta_\mu(z) \cr
    & = \S_i^\mu \hat{L}_a \Theta_\mu(z) 
\end{align}
If $\hat{L}_a \Theta = M_a \Theta$ (meaning 
$\hat{L}_a \Theta_\mu = [M_a]_\mu^\nu \Theta_\nu $), then we are staying in the same function basis $\Theta$. 
Then the equivariance condition becomes 
\begin{align}
    L_a' \S = \S M_a
    \label{eq:func-basis-cond}
\end{align}
We would like to have a systematic way to find a basis $\Theta(z)$ such that $\hat{L}_a \Theta = M_a \Theta$. 
This simplifies the symmetry condition \eqref{eq:inf-sym-cond} to a linear equation \eqref{eq:func-basis-cond}.
Next, we try to find a good basis $\Theta(z)$ such that \eqref{eq:func-basis-cond} can be satisfied and that the basis has some nice properties under the Lie algebra action. 

\subsection{Choosing function basis using the Lie algebra}
To get a linear equivariance condition \eqref{eq:func-basis-cond} we need to have 
\begin{align}
    \hat{L}_a \Theta (z) = M_a \Theta(z). 
    \label{eq:equiv-func-basis-LaMa}
\end{align}
If a row $\Theta_\mu(z) $ were an ``eigenfunction'' of $\hat{L}_a$, meaning $\hat{L}_a \Theta_\mu = \lambda_{ai} \Theta_\mu $, then making $\Theta$ the collection of eigenfunctions of $\hat{L}_a$ would naturally satisfy \eqref{eq:equiv-func-basis-LaMa}. 
We can do this for a fixed $a$, but we need \eqref{eq:equiv-func-basis-LaMa} for all $a$ and one fixed set of basis functions $\Theta$. 
Basic linear algebra states that for a non-abelian Lie algebra, a single basis $\Theta $ cannot be the eigenbasis for all $\hat{L}_a$. 
Nevertheless, it turns out that Lie algebras have some nice properties which allow us to choose a basis which satisfies \eqref{eq:equiv-func-basis-LaMa}. 
Specifically, as we review below, it suffices to find a common eigenbasis for the ``Cartan subalgebra'', which is the maximal commuting (Abelian) subalgebra $\mathfrak{h}\subset \mathfrak{g}$. 
This eigenbasis in fact includes the familiar Fourier basis for the Abelian translation group $G=(\R^n, +)$ and the Spherical harmonics for $SO(3)$. 

The reason that this becomes a closed basis for the whole $\mathfrak{g}$ is that the rest of the Lie algebra basis can be organized into operators which map one eigenfunction of each $\hat{L}_a \in \mathfrak{h}$ to another eigenfunction. 
These other $\hat{L}$ operators are often called raising and lowering operators, because they raise or lower the eigenvalues for the Cartan subalgebra by a fixed amounts. 
To provide some intuition, let us first look at a couple of examples:

\paragraph{Translation and the Fourier basis.}
The Translation group $\mathbf{T}_n = (\R^n,+)$ (real vectors under addition) acting on $\R^n$ can be represented as matrices of the form below acting on vectors in one higher dimensions $x' = (x|1)$ ($|$ meaning concatenation) for $x\in \R^n$  
\begin{align}
    && g &= \begin{pmatrix}
        I_n & \vec y \\ 
        \vec 0 & 1 
    \end{pmatrix} \in T_n, & 
    y &\in \R^n, & 
    gx' = \begin{pmatrix}
        x+y \\
        1
    \end{pmatrix} &&
\end{align}
The Lie algebra $\mathrm{Lie}(\mathbf{T}_n)$ is Abelian, with a canonical representation consisting of one-hot matrices $L_a = E_{n+1}^a$ ($[E^i_j]^k_l = \delta^{ik}\delta_{jl}$ is 1 at index $i,j$ and zero elsewhere). 
The flow operators $\hat{L}_a$ are given by

\begin{align}
    \hat{L}_a = [L_ax']^i\ro_i = \ro_a 
\end{align}
Now, let us find the eigenfunctions of $\hat{L}_a$ to choose as rows of $\Theta(x)$. 
We have 
\begin{align}
    \forall a \in \{1,\dots, n\}: \quad 
    \hat{L}_a \Theta_\mu & = \ro_a \Theta_\mu = \Lambda_{a \mu} \Theta_\mu, \cr 
    \Rightarrow \quad 
    \Theta_\mu &=  c_\mu \exp[\Lambda_{a\mu } x^a] = c_\mu \exp[\Lambda_{\mu}\cdot x]
\end{align}
where $\Lambda_{a\mu} \in \mathbb{C}$ is the eigenvalue for and $c_\mu $ is a normalization constant. 
When $\Lambda_{a\mu}$ has a real component, the function $\Theta_\mu $ diverges in some directions. 
Note that when $\Lambda$ is real we are dealing with the Laplace basis and when it is imaginary we have the Fourier basis. 
When dealing with symmetries in physical systems, such diverging functions are in some cases unphysical. 
In such cases, the Fourier basis is preferred, especially in quantum mechanics where we often model probability distributions with unitary dynamics (i.e., without dissipation). 
However, in other settings, such as the damped oscillator where dissipation is present we do need to consider $\Lambda$ with a nonzero real part. 

\paragraph{$SO(3)$, raising and lowering operators}
The Lie algebra $so(3)$ has structure constants equal to the 3D Levi-Cevita symbol $\eps_{ijk}$ which is completely anti-symmetric in its indices (i.e. equals zero when an index is repeated). 
For $a\in \{1,2,3\}$
\begin{align}
    L_a &\in so(3), &
    [L_a,L_b] &= \sum_c \eps_{abc} L_c, &
    \eps_{123}=1 &= - \eps_{213}.
\end{align}
Since no two of the basis $L_a$ commute, the Cartan subalgebra of $so(3)$ consists of just one of the $L_a$, traditionally chosen to be $h=L_3 \in \mathfrak{h}$ ($L_z$ in physics).
In physics, the basis of this Cartan algebra is traditionally chosen as $L_z = -i L_3$. 
Next, we want to find the basis functions $\Theta$ as eigenfunctions of $\hat{L}_z$. 
First, let us express this operator in the Cartesian basis and spherical coordinates $(r,\theta, \phi)$ where 
\begin{align}
    x &= \sin \theta \cos \phi \cr 
    y &= \sin \theta \sin \phi \cr 
    z &= \cos \theta  
\end{align}
We have 
\begin{align}
    L_3 &= \begin{pmatrix}
        0 & -1 &0 \\
        1 & 0 & 0 \\
        0 & 0 &0 
    \end{pmatrix}, &
    \hat{L}_z &= [-iL_3x]^i \ro_i = -i(x_1\ro_2 - x_2 \ro_1) = {-i\over r\sin \theta} \ro_\phi,  
\end{align}
where $\theta$ and $\phi$ are the polar and azimuthal angles.
For the eigenbasis to use in $\Theta$ we have 
\begin{align}
    \hat{L}_z \Theta_m &= {-i\over r\sin \theta} \ro_\phi \lambda_m \Theta_m, \cr 
    \Theta_m &= f_m(r,\theta) e^{im\phi}, \quad \hat{L}_z \Theta_m = m \Theta_m. 
    \label{eq:L3-Theta-basic}
\end{align}
\yjk{I believe $r\sin\theta$ shouldn't be in the denominator.
\begin{align}
    \partial_1 =& ... - \frac{\sin\phi}{r\sin\theta}\partial_\phi \cr
    \partial_2 =& ... + \frac{\cos\phi}{r\sin\theta}\partial_\phi \cr
    x_1\partial_2-x_2\partial_1 =& \partial_\phi
\end{align}
where $...$ are the $\partial_r$ and $\partial_\theta$ terms cancelling out.
}

Note that $\Theta$ should be continuous as $\phi$ crosses $2\pi$, meaning it must be periodic in $\phi$. 
That is why the exponent must be imaginary and why we chose $e^{im\phi}$. 
Additionally, note that with $L_3$ alone we do not have any constraints on $f_m(r,\theta)$. 
This is not desirable as it doesn't help us greatly in fixing the functional basis. 
We will come back to this below. 

The other two basis elements, $L_1$ and $L_2$ can be organized in the following way. 
The Lie algebra tells us that $[L_1,L_3] = -L_2$ and $[L_2,L_3]=L_1$. 
Hence we have 
\begin{align}
    L_\pm &\equiv L_1 \pm i L_2,& 
    [L_\pm, L_z ] & = \pm i L_\pm, &
    [L_+, L_- ] & = 2 L_z, 
    \label{eq:Lpm+-}
\end{align}
This means that $L_\pm$ can raise or lower eigenvalues for $L_3$ because 
\begin{align}
    L_z (L_\pm \Theta_m) &= \pm i L_\pm \Theta_m + L_\pm (L_z \Theta_m) = i(m \pm 1) L_\pm \Theta_m.
\end{align}
Thus, $L_\pm \Theta_m$ is in a subspace spanned by eigenfunctions $\Theta_{m\pm 1}$ of $L_z$, but the $f_m(r,\theta) $ part in this subspace may be mixing non-trivially. 
This means that, once we have chosen some basis for the subspace $\Theta_m$ (meaning $\Theta_m$ is not a single function, but all functions with different $f(r,\theta)$), we have 
\begin{align}
    L_\pm \Theta_m = M_m \Theta_{m\pm 1}
\end{align}
So, technically this basis satisfies our equivariance requirement \eqref{eq:equiv-func-basis-LaMa} because stacking $\Theta_m$ with different $m$, for all $a$ we have $L_a \Theta = M_m \Theta_m$. 
But this is still not satisfactory because we haven't fully resolved the basis $\Theta_m$ as $f_m$ is still unconstrained. 
But it turns out there are still other operators which commute with the Cartan subalgebra $\mathfrak{h}$, meaning they can help us alleviate the degeneraciy in $f_m$. 
This is precisely what is done in the representation theory of Lie algebra \nd{cite}.
Concretely, there exist ``Casimir operators'' which commute with all elements in the full algebra $\mathfrak{g}$ and hence also with $\mathfrak{h}$. 
In the case of $so(3)$ we have the ``total angular momentum'' operator, which is the quadratic Casimir 
\begin{align}
    C= L^2 = \sum_a L_a^2
\end{align}
Finding a common eigenbasis for $\hat{L}_z$ and $\hat{L}^2$ yields the familiar spherical harmonics $Y_l^m$ satisfying 
\begin{align}
    Y_l^m &= e^{im\phi} P_l^m(\cos \theta) \cr 
    \hat{L}_z Y_l^m& = mY_l^m, \cr
    \hat{L}^2 Y_l^m &= l(l+1) Y_l^m,
\end{align}

\paragraph{Quadratic Casimir operator}
When trying to define the function basis $\Theta$ it is desirable to have as many commuting linear operators as possible. 
More operators means more constraints on the basis and less arbitrary choices. 
It allows us to resolve degeneracies, refine the basis. 
Note that in addition to the basis elements $L_a$, there can be other operators which commute with $L_3$ and which can help us refine the basis $\Theta$. 
Specifically, one such object is the quadratic Casimir operator (an element of the ``universal enveloping algebra'' of a Lie algebra \nd{cite}). 
In the case of $SO(n)$ the Casimir operator simply becomes 
\begin{align}
    C = \sum_a L_a^2, \quad \forall a: [C,L_a] = 0
\end{align}
Note that the Casimir operator also becomes the Laplacian in euclidean when working with the operator representation $\hat{L}_a$: 
\nd{Working on it}

\paragraph{Using the eigenbasis of the Cartan subalgebra.}
% Under what conditions does this happen? 
% Or rather, does there exist a basis $\Theta$ such that $\hat{L}_a \Theta = M_a \Theta$? 
The eigenbasis of the Cartan subalgebra (maximal abelian subalgebra for finite-dimensional semisimple groups) may help us here. 
Let $\mathfrak{h}\subseteq \mathfrak{g}$ be the Cartan subalgebra where 
\begin{align}
    \forall h_a, h_b \in \mathfrak{h}, \qquad [h_a,h_b] = 0
\end{align}
Since all $h_a \in \mathfrak{h}$ commute, 
we can find a common eigenbasis for them. 
Also, there exists a Casimir operator $C$ which also commutes with all $L_a \in \mathfrak{g}$ and so it can be diagonalized simultaneously with all of $\mathfrak{h}$. 
% Note that the Lie algebra of $L_a$ induces the same Lie algebra on the vector fields $\hat{L}_a$ because 
% \begin{align}
%     [\hat{L}_a, \hat{L}_b]=...
% \end{align}
Semisimple Lie algebras have a root system decomposition where the Lie algebra basis can be decomposed into elements $T\in \mathfrak{g}$ such that  %$\mathrm{ad}(h)L = [h,L] = \alpha(h) L$.
\begin{align}
    \forall h \in \mathfrak{h}, \qquad 
    [h,T] = \alpha(h) T
\end{align}
This is similar to an eigenvalue equation. 
The ``roots'' $\alpha(h)$ have the property that $-\alpha(h)$ is also as a root. 
Due to this, the $T$ can be organized into raising and lowering operators, $T_{\pm}$ such that 
\begin{align}
    [h,T_+] = \alpha(h) T_+, \qquad 
    [h,T_-] = -\alpha(h) T_-, 
\end{align}
Using the Jacobi identity (see \eqref{eq:hT+-Jacobi}) we can show that $T_0 = [T_+,T_-]$ is also in the Cartan subalgebra $\mathfrak{h}$, since 
\begin{align}
    [h,T_0]=[[h,T_+],T_-]+[[T_-,h],T_+] = 0
\end{align}
% which means $T_0 = [T_+,T_-]$ is in the Cartan subalgebra. 
Thus, $[T_0, T_\pm]= \pm \alpha(T_0)T_\pm$.  
There are simple roots, which are positive and cannot be written as the sum of other simple roots.
Then, if we look for eigenfunctions of $\hat{h}$, the simple roots would change these eigenfunctions to each other as raising/lowering operators because 
\begin{align}
    \hat{h} Y &= \lambda(h) Y, &
    \hat{h}[\hat LY] &= (\alpha(h)+\lambda(h))[\hat{L} Y]
    \label{eq:hY-eigfunc}
\end{align}
meaning $\hat L Y$ is a new eigenfunction of $\hat h$ with eigenvalue $\lambda+\alpha$.
% What does this tell us? 

We were looking for a choice of $\Theta(z) $ that is guaranteed to satisfy the equation $\hat{L}_a \Theta = M_a \Theta$. 
\eqref{eq:hY-eigfunc} reveals that we can choose $\Theta$ to be the set of eigenfunctions $Y_\lambda$ of $\mathfrak{h}$ with eigenvalue $\lambda(h)$ for $h \in \mathfrak{h}$.
\nd{More simply, because all of $\mathfrak{g}$ commutes with identity, we can choose $\Theta$ to be eigenfunctions of the flow induced by the identity element, which turns out to be the scaling operator because
\begin{align}
    \hat{id} = [Iz]^T \grad = z^i\ro_i
\end{align}
The eigenfunctions of the scaling operator $\hat{id}$ are simply homogeneous functions of a fixed order. 
Thus, we can always choose $\Theta$ to be such homogeneous functions. 
}

The whole Lie algebra $\mathfrak{g}$ can be decomposed into (Serre Theorem? Serre relations) into 
\begin{align}
    \mathfrak{g} = \mathfrak{h} \bigoplus_\alpha \mathfrak{g}_\alpha 
\end{align}
It follows that the set of all eigenvectors of $\hat{\mathfrak{h}}$ can form an eigenbasis for $\mathfrak{h}$. 
This is because the rest of the Lie algebra basis become raising an lowering operators which change the eigenvalues by $\alpha(h)$. 
Thus, if all eigenfunctions are in $\Theta$, acting with $L_\alpha $ on $\Theta$ will only switch the rows with a circulant matrix $C_\alpha$ which shifts the rows by $\alpha$, meaning 
\begin{align}
    L_\alpha \Theta = C_\alpha \Theta 
\end{align}
Hence, choosing $\Theta $ to be eigenfunctions of $\hat{\mathfrak{h}}$ exactly satisfies the relation we need for equation discovery. 
The question is in terms of simplicity of equations and interpretability, is this a good choice or not.

\nd{
\paragraph{More general linear dynamics.}
What if we have a field theory? 
Let $\phi: \mathcal{Z} \to \mathcal{V} $ be a ``field''.

}

\nd{Does this vector field form $\hat{L}=[Lz]^T\grad $ naturally result in a commutator-Poisson brackets relation? 
In other words, can the commutator naturally be rewritten as a Poisson brackets if we replace $\ro_i\to p_i$? 
This could be done for a general operator $F(z,\ro) = F(z,p) $. 
Observe that (make accurate; needs Moyal brackets and $e^{i/\hbar S}$ and expansion to first order in $\hbar$. )
\begin{align}
    [z,\ro ]h &= -[\ro,z]h = z\ro h - \ro(zh) = -h\cr 
    [F,G]h &= {\ro F\over \ro z}{\ro G\over \ro p}[z,\ro]h + {\ro F\over \ro p}{\ro G\over \ro z}[\ro,z]h\cr 
    &= {\ro F\over \ro p}{\ro G\over \ro z}h-{\ro F\over \ro z}{\ro G\over \ro p}h = -\{F,G\}h
\end{align}
}

\section{Derivations: Equivariant equations \label{ap:derivations-equiv-eq} }

\nd{When $K$ commutes with $L_a$, what can we say about it? 
It doesn't have to be a Casimir operator or in the Cartan subalgebra, right? 
But it may restrict how to choose Cartan, maybe? 
What about the nonlinear version $h(z)$? 
Can we somehow relate it to some infinitesimal group action? 
Maybe if it was a PDE? Basically, I wonder if $h(z) $ could also be restricted to related to Casimir or Cartan, maybe in the tangent space. 
}

Let $z\in \mathcal{Z}\sim \R^k$ be the latent space.
Let $\pi: G\to \GL(\mathcal{Z})$ be a representation of $G$ defining a linear action on $\mathcal{Z}$ as 
\begin{align}
    g\cdot z = \pi(g) z.
\end{align}
Pick a group element $g \in G$ close to identity such that  $\pi(g) = I+\eps\cdot L= I+\eps^a L_a$, with $L_a \in \mathfrak{g}= T_IG$ as the Lie algebra basis.
When $G $ is a symmetry of the dynamics, it must commute with the dynamics $d/dt$, meaning 
\begin{align}
    \mbox{Symmetry of dynamics: }
    g\cdot {d z\over dt }= {d(g\cdot z)\over dt}.
\end{align}
Let the dynamics be $\dot{z}= dz/dt=h(z)$. 
\nd{In principle $z$ and $\dot z$ can transform under different reps. Ex: when $z\in [0,2\pi)$ is the pendulum angle, $dz/dt\in \R$ is not necessarily in the same space!} 
% (Einstein summation). 
% \paragraph{Case 1: $z$ and $\dot{z}$ share rep.}
% Assuming $\dot z \in \mathcal{Z}$, we can assume that $\dot{z}$ transforms with the same representation $\pi$ as $z$ did. 
% \begin{align}
%     \pi(g) \dot{z} &= h(\pi(g) z) \cr
%     (I+\eps \cdot L) \dot z &= h((I+\eps\cdot L)z) \cr 
%     &= h(z) + [\eps\cdot Lz]^i \ro_i h(z) + O(\eps^2)\cr 
%     \Rightarrow L_a\dot z&=[L_az]^T \grad h(z)
% \end{align}
% \paragraph{Case 2: $z$ and $\dot{z}$ share rep.}

$\dot z$ and $z$ are not always in the similar space and do not necessarily transform the same way. 
For instance, for a pendulum, $z$ can be the angle, meaning $z\in [0,2\pi)$, while $\dot{z}\in \R$.  
Let $\dot z \in \mathcal{Z}'$ transform with representation $\pi':G \to \GL(\mathcal{Z}')$. 
Denote the representations of a small element by $\pi(g) = I+\eps L$ and $\pi'(g) = I+\eps L'$.
We have 
\begin{align}
    \pi'(g) \dot{z} &= h(\pi(g) z) \cr
    (I+\eps \cdot L') \dot z &= h((I+\eps\cdot L)z) \cr 
    &= h(z) + [\eps\cdot Lz]^i \ro_i h(z) + O(\eps^2)\cr 
    \Rightarrow L_a'\dot z&=[L_az]^T \grad h(z) 
    \label{eq-ap:Lz-dyn-sym}
\end{align}
Defining the linear operator (vector field in $T\mathcal{Z}$). 
\begin{align}
    \hat{L}_a(z) \equiv [L_az]^i \ro_i  
\end{align}
the dynamics symmetry condition \eqref{eq-ap:Lz-dyn-sym} becomes 
\begin{align}
    L_a h(z) &= \hat{L}_a h(z). 
\end{align}

\paragraph{Lie algebra of $\hat{L}_a$.}
Note that $\hat{L}_a$ satisfy a Lie algebra similar to that of $L_a$. 
Denote the Lie bracket relations by 
\begin{align}
    [L_a,L_b] = {f_{ab}}^c L_c
\end{align}
where ${f_{ab}}^c$ are the structure constants. 
We have 
\begin{align}
    \hat{L}_a \hat{L}_b h(z)&= [L_az]^T\grad \pa{[L_bz]^T \grad h} \cr 
    &=[L_az]^i\ro_i[L_bz]^j \ro_j h + [L_az]^i[L_bz]^j \ro_i\ro_j h \cr 
    [L_az]^i\ro_i[L_bz]^j \ro_j h &= [L_a]^i_kz^k [L_b]^j_l \ro_iz^l \ro_j h \cr 
    &=[L_a]^i_kz^k [L_b]^j_l \delta_i^l \ro_j h \cr 
    &=[L_a]^i_kz^k [L_b]^j_i  \ro_j h \cr 
    &=[L_bL_az]^T \grad h. 
    \label{eq:LaLb-Lie-alg}
\end{align}
The $[L_a]^i_kz^k [L_b]^j_l \ro_iz^l \ro_j f$ term is symmetric under $a\leftrightarrow b$ and cancels in the two terms from the commutator. \yjk{Do you mean the second term, $[L_az]^i[L_bz]^j\partial_i\partial_jh$? We may need some conditions for a symmetric Hessian matrix $\partial_i\partial_jh$, e.g. continuous second partial derivatives.}
Thus, we get
\begin{align}
    [\hat{L}_a, \hat{L}_b]h &= \br{[L_b,L_a]z}^T \grad h \cr 
    & = {f_{ba}}^c\br{L_cz}^T \grad h \cr 
    &= -{f_{ab}}^c \hat{L}_c h
\end{align}
which is the same as the algebra satisfied by $L_a^T$
\begin{align}
    [L_a^T,L_b^T]&=[L_b,L_a]^T = {f_{ba}}^c L_c^T = -{f_{ab}}^c L_c^T. 
\end{align}

\nd{Because of the similar Lie algebra, maybe we can express some conditions on the dynamics $h(z)$ in terms of Linear differential operators. 
For example, instead of the simple linear dynamics $h=Kz$ where $K\in \R^{n\times n}$, we could have $h=\hat{K}z$ where $K \in T\mathcal{Z}$ is a differential operator. 
Then, maybe symmetry condition with $L=L'$ dictates that $\hat{K}$ must commute with $\hat{L}_a$, which makes it a Casimir operator? 
}

\paragraph{Example: Linear.}
In the linear case $h(z) =Kz$ we have 
\begin{align}
     [L_a' K z]_j&=
     [L_a z]^i  K_{jl} \ro_i z^l %\cr &= [L_a z]^i K_{jl} \delta_i^l = [L_a z]^i K_{ji} 
     = [KL_a z]_j\cr 
     \Rightarrow L_a' K &= KL_a
     \label{eq:KL-linear}
\end{align}
which means that $K$ has to be an intertwiner between $\pi$ and $\pi'$.  
Assuming $z$ and $\dot{z}$ transform the same way ($\pi=\pi'$), \eqref{eq:KL-linear} becomes $L_a K= KL_a$, or $[K,L_a]=0$. 

\paragraph{General dynamics.}
Define the linear operator 
\begin{align}
    \hat{L}_a(z) \equiv [Lz]^i \ro_i  
\end{align}
The dynamics symmetry condition  
which defines a vector field (or flow) on $\mathcal{Z}$.  
Express $h(z) = \S \Theta(z)$ in terms of some function basis $\Theta(z)$. 
We get
\begin{align}
    L_a' h(z) &= \hat{L}_a h(z) \cr 
    [L_a' \S \Theta]_i &=[L_a']_i^j\S_j^\mu \Theta_\mu  \cr 
    & = [L_a z]^k \ro_k \S_i^\mu \Theta_\mu(z) \cr 
    & = \S_i^\mu [L_a z]^k \ro_k \Theta_\mu(z) \cr
    & = \S_i^\mu \hat{L}_a \Theta_\mu(z) 
\end{align}
If $\hat{L}_a \Theta = M_a \Theta$ (meaning 
$\hat{L}_a \Theta_\mu = [M_a]_\mu^\nu \Theta_\nu $), then we are staying in the same function basis $\Theta$. 
Then the equivariance condition becomes 
\begin{align}
    L_a \S = \S M_a
\end{align}
Under what conditions does this happen? 
Or rather, does there exist a basis $\Theta$ such that $\hat{L}_a \Theta = M_a \Theta$? 
The eigenbasis of the Cartan subalgebra (maximal abelian subalgebra for finite-dimensional semisimple groups) may help us here. 
Let $\mathfrak{h}\subseteq \mathfrak{g}$ be the Cartan subalgebra where 
\begin{align}
    \forall L_a, L_b \in \mathfrak{h}, \quad [L_a,L_b] = 0
\end{align}
Since all $L_a \in \mathfrak{h}$ commute, 
we can find a common eigenbasis for them. 
Also, there exists a Casimir operator $C$ which also commutes with all $L_a \in \mathfrak{g}$ and so it can be diagonalized simultaneously with all of $\mathfrak{h}$. 
% Note that the Lie algebra of $L_a$ induces the same Lie algebra on the vector fields $\hat{L}_a$ because 
% \begin{align}
%     [\hat{L}_a, \hat{L}_b]=...
% \end{align}
Semisimple Lie algebras have a root system decomposition where $\mathrm{ad}(h)L = [h,L] = \alpha(h) L$. 
This is kind of similar to an eigen-decomposition. 
Since the roots $\alpha(h)$ will always have $-\alpha(h)$ also as a root, these are like raising and lowering operators.

From the Jacobi identity we have 
\begin{align}
    &[h,[T_+,T_-]]+[T_-,[h,T_+]]+[T_+,[T_-,h]]=0 \cr 
    &[h,[T_+,T_-]]+[T_-,\alpha T_+]+[T_+,\alpha T_-]=0 \cr 
    & [h,[T_+,T_-]] =0,\qquad \Rightarrow\qquad [T_+,T_-] \in \mathfrak{h}  
    \label{eq:hT+-Jacobi}
\end{align}

There are simple roots, which are positive and cannot be written as the sum of other simple roots.
Then, if we look for eigenfunctions of $\hat{h}$, the simple roots would change these eigenfunctions to each other as raising/lowering operators because 
\begin{align}
    \hat{h} Y &= \lambda Y, &
    \hat{h}[\hat LY] &= (\alpha(h)+\lambda)[\hat LY]  
\end{align}
meaning $\hat L Y$ is a new eigenfunction of $\hat h$ with eigenvalue $\lambda+\alpha(h)$.
What does this tell us? 
We wanted to see if a particular choice of $\Theta(z) $ is guaranteed to satisfy the equation $\hat{L}_a \Theta = M_a \Theta$. 
Let's choose $\Theta$ to be the set of eigenfunctions $Y_\lambda$ of $\mathfrak{h}$ with eigenvalue $\lambda(h)$ for $h \in \mathfrak{h}$.
The whole Lie algebra $\mathfrak{g}$ can be decomposed into (Serre Theorem? Serre relations) into 
\begin{align}
    \mathfrak{g} = \mathfrak{h} \bigoplus_\alpha \mathfrak{g}_\alpha 
\end{align}
It follows that the set of all eigenvectors of $\hat{\mathfrak{h}}$ can form an eigenbasis for $\mathfrak{h}$. 
This is because the rest of the Lie algebra basis become raising an lowering operators which change the eigenvalues by $\alpha(h)$. 
Thus, if all eigenfunctions are in $\Theta$, acting with $L_\alpha $ on $\Theta$ will only switch the rows with a circulant matrix $C_\alpha$ which shifts the rows by $\alpha$, meaning 
\begin{align}
    L_\alpha \Theta = C_\alpha \Theta 
\end{align}
Hence, choosing $\Theta $ to be eigenfunctions of $\hat{\mathfrak{h}}$ exactly satisfies the relation we need for equation discovery. 
The question is in terms of simplicity of equations and interpretability, is this a good choice or not.
