# Supplementary material for: Symmetry-Informed Governing Equation Discovery
Source: arXiv:2405.16756 source file (2024-11-04)
Supplement: Supplementary file 3 [file tds.tex]

\section{Reformulation for Time-Dependent Symmetries}
\subsection{ODE}
We consider first-order ordinary differential equations of the following form:
\begin{equation}
\label{eq:ode0}
    \frac{d\bm x}{dt} =\bm h(t, \bm x)
\end{equation}
where $t$ denotes time, i.e. the only independent variable in ODEs, and $\bm x \in X \simeq \R^n$ denotes the dependent variables. Our goal is to discover the function $\bm h$ in a symbolic form from the observed trajectories of the system. We may assume some additional restrictions on the form of $\bm h$, e.g. it does not explicitly depend on time. For now, we consider its most general form.

To formalize the concept of symmetries, we take a geometric perspective on the differential equations \eqref{eq:ode0}. The independent and the dependent variables form a total space $E = T \times X$. We define the first-order jet space of the total space as $\mathcal J = T \times X \times X_1$. Its coordinates, $(t, x_1, ..., x_n, x'_1, ..., x'_n) \in \mc J$, represent the independent and the dependent variables as well as the time derivatives of the dependent variables. This is also known as the first-order \textbf{prolongation}.

Then, we can represent the ODE \eqref{eq:ode0} through the map $\Delta: \mc J \to \R^n$ with components $\Delta_i = x'_i - h_i(t, \bm x)$. A function $\bm x(t)$ is a solution of \eqref{eq:ode0} if its prolongation satisfies
\begin{equation}
\label{eq:ode1}
    \Delta (t, \bm x, \bm x')=0
\end{equation}

\subsection{Symmetry}
A symmetry of the system $\Delta$ transforms one of its solutions to another. More specifically, we need to define the group action on a point in the total space $E = T \times X$ and its induced action on a function $T \to X$.

We express the action of group element $g$ in the total space as
\begin{equation}
    g\cdot(t, \bm x) = (\hat t(t, \bm x), \hat {\bm x}(t, \bm x)),
\end{equation}
where $\hat t$ and $\hat {\bm x}$ are functions over $T \times X$.

To define the induced group action on the function $f: T \to X$, we first identify $f$ with its graph
\begin{equation}
    \gamma_f = \{ (t, f(t)): t \in \Omega_T \} \subset T \times X
\end{equation}
where $\Omega_T \subset T$ is the time domain. The graph of the function can be transformed by $g$ as
\begin{equation}
    g \gamma_f = \{ (\tilde t, \tilde {\bm x}) = g\cdot(t, \bm x): (t, \bm x) \in \gamma_f \}
\end{equation}

The set $g \gamma_f$ may not be the graph of another single-valued function. However, by choosing a suitable domain $\Omega_T$, we ensure that the group elements near the identity transform the original graph into a graph of some other single-valued function $\tilde x = \tilde f(\tilde t)$ with the transformed graph $\gamma_{\tilde f} = g\cdot \gamma_f$. In other words, the transformed function $\tilde f = g\cdot f$ is defined by the transformation of the function graph.

\begin{definition}[Def 2.23, \cite{olver1993applications}]\label{def:ode-symm}
    A symmetry group of $\Delta$ \eqref{eq:ode1} is a local group of transformations $G$ acting on an open subset of the total space $T \times X$ that whenever $\bm x = f(t)$ is a solution of $\Delta$, and whenever $g\cdot  f$ is defined for $g \in G$, then $ {\bm x} = (g\cdot f)( t)$ is also a solution of the system.
\end{definition}

\subsection{The Infinitesimal Criterion}
Let $\bm v$ be a vector field on the total space $T \times X$ with corresponding one-parameter subgroup $\exp (\epsilon \bm v)$. The vector field describes the infinitesimal transformations to the independent and the dependent variables. It can be written as
\begin{equation}
\label{eq:vf}
    \bm v(t, \bm x) = \xi(t, \bm x)\partial_t + \sum_i \phi^{i}(t, \bm x)\partial_{x_i}.
\end{equation}

\yjk{We may have different assumptions about the vector field. In our original submission, all transformations are time-independent, i.e. $\xi = 0$. We also assume that nonlinear $\phi$ can be decomposed into an encoder-linear-action-decoder structure if we use LaLiGAN. These restrictions can be lifted to represent more general forms of symmetries. In particular, we observe that many differential equations have time-dependent symmetries, and the vector fields can be written in symbolic form. This motivates us to (1) include the $\xi$ component and (2) use symbolic model for all the components instead of the LaLiGAN architecture. For (2), we will also need an alternative procedure to matrix exponential to integrate the vector field into a finite transformation.}

The vector field also has its induced infinitesimal action on the jet space $T \times X \times X_1$ described by the \textbf{prolonged vector field}:
\begin{equation}
    \bm v^{(1)} = \bm v + \sum_i \phi_i^{(1)}(t,\bm x, \bm x')\partial_{x'_i}
\end{equation}
where $\phi_i^{(1)}$ can be computed by the \textit{prolongation formula} as
\begin{align}
    \phi_i^{(1)} = & D_t [\phi_i - \xi x_i'] + \xi x''_i
    \\
    = & \pd{\phi_i}{t} + \sum_j x'_j\frac{\partial \phi_i}{\partial x_j} - x'_i \big(\pd{\xi}{t} + \sum_j x'_j\frac{\partial\xi}{\partial x_j}\big)
\end{align}

\yjk{Note: the prolongation can be computed for higher-order jet spaces as well. However, as we only consider first-order ODEs in this paper, we only need to compute the prolonged vector field on $T\times X\times X_1$.}

Specifically, for the time-independent symmetries we considered previously, $\xi=0$ and $\phi(t, \bm x) = \phi(\bm x)$, so we have
\begin{equation}
\label{eq:prv-ti}
    \phi_i^{(1)} = \sum_j \frac{\partial \phi_i}{\partial x_j} x'_j
\end{equation}

Another special case is time translation. When $\xi = 1$ and $\phi = 0$, we have $\phi_i^{(1)} = 0$.

The infinitesimal criterion indicates the symmetry condition in terms of the vector field (and its prolongation). It is the analog of \cref{th:inf_constraint} when we generalize the notion of symmetry.
\begin{theorem}[The infinitesimal criterion. Thm 2.31, \cite{olver1993applications}]\label{th:lps-inf}
    Let $\Delta$ be a system of ODEs of maximal rank defined over $M \subset T \times X$. A local group of transformations $G$ acting on $M$ is a symmetry group of the system $\Delta$ iff \footnote{Strictly speaking, the reverse only holds when $\Delta$ satisfy certain additional local solvability conditions.} for every infinitesimal genrator $\bm v$ of $G$, $\bm v^{(1)}[\Delta_i] = 0$, $i=1, ..., n$, whenever $\Delta = 0$.
\end{theorem}

Once we have the symmetry represented by the vector field $\bm v$, we can derive constraints on the equation form from the above theorem.

Generally, when the vector field takes the general form in \eqref{eq:vf}, we can enforce \cref{th:lps-inf} by its equivalent condition
\begin{equation}
    J_{\bm\phi}(t) + J_{\bm\phi}(\bm x)\bm h(\bm x) - (\xi_t + (\nabla_{\bm x}\xi)^T\bm h(\bm x))\bm h(\bm x)
    = \bm \phi^{(1)}(t, \bm x, \bm h(\bm x))
    = J_{\bm h}(t, \bm x)\begin{bmatrix}
        \xi(t, \bm x) \\ \bm \phi(t, \bm x)
    \end{bmatrix}
\end{equation}

More specifically, when we assume time-independent symmetries and thus the prolonged vector fields given by \eqref{eq:prv-ti}, the symmetry condition \cref{th:lps-inf} is equivalent to
\begin{equation}
    \sum_j \pd{\phi_i}{x_j}x'_j = \sum_j \pd{h_i}{x_j}\phi_j,\quad i=1,...,n
\end{equation}
or, in its matrix form, $J_{\bm v}(\bm x)\bm h(\bm x) = J_{\bm h}(\bm x)\bm v(\bm x)$. (Note that if we define $\bm \phi = [\phi_1, ..., \phi_n]^T$, then $\bm \phi(\bm x) = \bm v(\bm x)$, leading to this matrix expression with $\bm v$ instead of $\bm \phi$.)

\yjk{Therefore, an obvious solution to symmetry is $\bm v = \bm h$. The symmetry generated by this vector field, $g = \exp(\epsilon \bm v)$, acts like time translation although it is not directly transforming the time, in the sense that $(g \cdot \bm x)(t) = \bm x(t + \epsilon)$.}

On the other hand, we can also convert the constraint on the flow map $\bm f_\tau \coloneqq \exp(\tau\bm h)$ in \cref{th:inf_constraint} into the constraint on $\bm h$. By applying $\od{}{\tau}|_{\tau=0}$ to both sides of the equation, we have
\begin{align}
    & J_{\bm f_\tau}(\bm x)\bm v(\bm x) = \bm v(\bm f_\tau (\bm x)) \label{eq:inf-symm-fl} \\
    \Rightarrow & \Big(\od{}{\tau}\Big|_{\tau=0} J_{\bm f_\tau}(\bm x) \Big)\bm v(\bm x) = J_{\bm v}(\bm f_{\tau=0}(\bm x))\Big(\od{}{\tau}\Big|_{\tau=0}\bm f_\tau (\bm x)\Big) \\
    \Rightarrow & J_{\bm v}(\bm x)\bm h(\bm x) = J_{\bm h}(\bm x)\bm v(\bm x) \label{eq:inf-symm-vf}
\end{align}
which shows that \cref{th:inf_constraint} is a special case of \cref{th:lps-inf} when the vector field only acts on the dependent variables $\bm x$ without involving time $t$.

If we further assume both $\bm h$ and $\bm v$ can be expressed in symbolic terms as $\bm h(\bm x) = W\Theta(\bm x)$ and $\bm v(\bm x) = U\Theta(\bm x)$, the constraint on $W$ (given $U$) becomes
\begin{equation}
    UJ_\Theta(\bm x)W = WJ_\Theta(\bm x) U, \quad \forall \bm x
\end{equation}

\subsection{Equivariance of Flow Map}
The previous discussion gives us the following proposition.

\begin{proposition}
If the flow map $\bm f_\tau \coloneqq \exp (\tau\bm h)$ of the ODE $\dot {\bm x} = \bm h(\bm x)$ is equivariant to the one-parameter subgroup $\exp (\epsilon \bm v)$ with respect to the group action $g: X \to X$, then $\exp (\epsilon \bm v)$ is a symmetry group of the ODE in terms of \cref{def:ode-symm} and the group action given by point transformation on the total space $g: (t, \bm x) \mapsto (t, g\cdot \bm x)$.
\end{proposition}

\begin{proof}
From \cref{th:inf_constraint}, we have \eqref{eq:inf-symm-fl} and thus \eqref{eq:inf-symm-vf}. From \cref{th:lps-inf}, we know that $\exp (\epsilon \bm v)$ is a symmetry group of the ODE system.
\end{proof}

That is, the equivariance of the flow map is a sufficient condition for a time-independent Lie point symmetry of the ODE. However, the converse is not generally true. The flow map is not necessarily equivariant to the point transformations of a symmetry group of the ODE, even if the transformations leave the time invariant. To understand this, note that the deduction from \eqref{eq:inf-symm-fl} to \eqref{eq:inf-symm-vf} is not invertible. Consider the following counterexample.

% \begin{example}
%     Consider the first-order ODE given by $\dot{\bm x} = (-x_2/r, x_1/r)^T$, where $\bm x \in \R^2$ and $r = \sqrt{x_1^2+x_2^2}$. The solution trajectories are circles centered at the origin. The solutions move along the circles at unit speed. Thus, the flow map can be analytically expressed as $\bm f_\theta: (a\cos \theta_0, a\sin \theta_0) \mapsto (a\cos (\theta+\theta_0), a\sin (\theta+\theta_0))$.

%     A symmetry group of this system is the scaling symmetry $g_a: (t, \bm x) \mapsto (t, a\bm x)$

%     Consider the trajectory starting at $x_0 = (1,0).$
% \end{example}

\subsection{Discovering Lie Point Symmetries}
The solution set of the differential equations $\Delta$ is given by
\begin{equation}
    \textrm{Sol}_\Delta = \{ f: T \to X\, | \, \Delta(t, f(t), f'(t)) = 0 \}
\end{equation}

For symmetry discovery, we want to find transformations that leave the solution set invariant. Similar to our previous approaches, we label the observations from the dataset as positive samples and the transformed observations as negative ones, and perform adversarial training. However, there are also differences from previous settings.

\paragraph{The vector field.}
The vector field $\bm v$ in the context of Lie point symmetries is analogous to the Lie algebra representation (the $L_i$ matrices) in our previous papers. When $\bm v$ is linear, we can use the matrix exponential to compute the finite transformation. Generally, $\bm v$ contains nonlinear terms, so we need another way to integrate the infinitesimal action to a finite one. Also, the vector fields can be expressed analytically. This motivates us to create a symbolic model for the vector field instead of the encoder-linear-rep-decoder architecture in LaLiGAN. Once we have a analytical vector field, we can enforce the infinitesimal constraint instead of using it as a regularizer.

\paragraph{Representing the solution.}
Note that the elements in $\textrm{Sol}_\Delta$ are functions. As we mention earlier, these solutions are the input to the symmetry generator and the discriminator. Thus, we need a proper way to represent these functions. A natural choice is to evaluate it at regular time interval, e.g. $(f(t_0), f(t_0+\Delta t), ..., f(t_0+(T-1)\Delta t)) \in \R^{n \times T}$.

A problem arises when we try to learn time-dependent symmetry transformations. As the group acts on the function via its graph, the resulting representation of $\tilde f \coloneqq g\cdot f$ would become $(\tilde f(\tilde t_0), ..., \tilde f(\tilde t_{T-1}))$. We may need to resample the transformed representation to temporally align it with the original sample.

\newpage
